# Supplementary material for: Optomechanical Anti-lasing with Infinite Group Delay at a Phase Singularity
Source: arXiv:2112.06521 ancillary file (2021-12-13)
Supplement: Supplementary file 1 [file Supplementary-Material.pdf]

# Supplementary information for “Optomechanical Anti-lasing with Infinite Group Delay at a Phase Singularity”

Yulong Liu,[1,2] Qichun Liu,[1] Shuaipeng Wang,[3]
Zhen Chen,[1] Mika A. Sillanpää,[2,*] and Tiefu Li[4,1,†]

[1]*Beijing Academy of Quantum Information Sciences, Beijing 100193, China*

[2]*Department of Applied Physics, Aalto University, P.O. Box 15100, FI-00076 Aalto, Finland*

[3]*Quantum Physics and Quantum Information Division, Beijing Computational Science Research Center, Beijing 100193, China*

[4]*School of Integrated Circuits and Frontier Science Center for Quantum Information, Tsinghua University, Beijing 100084, China*

(Dated: December 13, 2021)

This supplementary material is organized as follows: Sec. I describes the 3D superconducting cavity electromechanical device. In Sec. II, we simulate the electric field distributions with an antenna inside the 3D cavity. In Sec. III, the measurement setups are presented. In Sec. IV, the theoretical calculations show the $\pi$-phase transition and group-delay singularity. The calibrations of the system parameters and optomechanical coupling strength are presented in Sec. V. Sec. VI presents the measured group delay for a continuous probe-field generated from the VNA.

**CONTENTS**


I. 3D-superconducting cavity electromechanical device 2

II. Electromagnetic-field distributions inside the 3D-superconducting cavity 4

III. Measurement setups 6

IV. Simulation of the $\pi$-phase transition 8

V. Device parameters and the optomechanical coupling strength 14

VI. Group delay measurements by the VNA 15

References 16


## I. 3D-SUPERCONDUCTING CAVITY ELECTROMECHANICAL DEVICE

The whole 3D superconducting cavity electromechanical device is shown in Fig. S1(a). The mechanically compliant capacitor chip is placed at the center of the rectangular Al-box and capacitively coupled to the cavity mode. Compared to direct galvanic coupling through indium foil extrusion [1], the wireless connection between a mechanical compliant capacitor and 3D cavity can effectively avoid any unexpected external force disturbance and uneven stress distribution for the SiN membrane. Huge capacitances $C_p$ are formed between the antenna electrode and the cavity wall. These two large capacitors are connected in series in the circuit.

The packaged mechanical-compliant-capacitor chip is shown in Fig. S1(b). The equivalent lumped parameter model for the electromechanical device is then given in Fig. S1(c). The capacitors ($C_p$) between the 3D cavity and the antenna are much larger than the mechanical capacitor

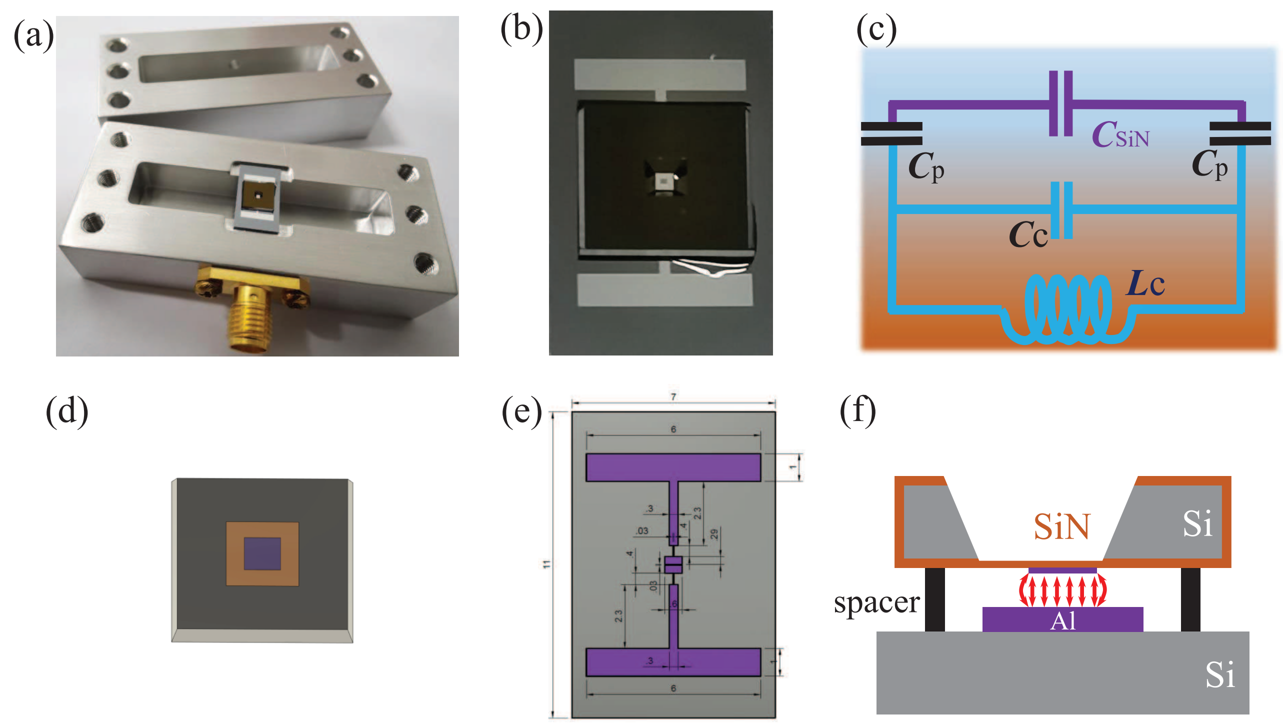


FIG. S1. (a) The 3D superconducting cavity electromechanical device. (b) Packaged mechanically compliant capacitor chip. (c) The equivalent lumped parameter model for the electromechanical device. (d) The metalized SiN-membrane chip. (e) The antenna chip and its detailed size parameters. (f) The schematic diagram shows the side-view of the assembled mechanically compliant capacitor. The aluminum films (marked in purple) are deposited by an electron-beam-evaporator. The Al-film thicknesses are 20-nm and 120-nm for the SiN and bottom antenna chips, respectively. Epoxy-pillars are used to bond the upper and lower two chips.

($C_{\mathrm{SiN}}$) and cavity capacitor ($C_{\mathrm{C}}$). Thus, the wireless connection between the antenna and the 3D cavity is equivalent to a galvanic connection by shorting antennas to the cavity wall. Thus, the wireless connection allows a relatively high single-photon coupling strength while introducing the minimum stress disturbance for the SiN membrane.

We now discuss the detailed structure of the packaged mechanical-compliant-capacitor chip as shown in Fig. S1(b). It is assembled from a metalized SiN-membrane chip and an antenna chip. Figure. S1(d) shows a 5 mm$\times$5 mm$\times$0.5 mm chip with a released SiN membrane. The membrane size is 500 $\mu$m$\times$500 $\mu$m$\times$50 nm. High stress (800 Mpa) is evenly distributed in the membrane plane to increase the mechanical mode frequency and Q value. The SiN membrane is then metalized through e-beam evaporation. An aluminum square with 200 $\mu$m wide and 20 nm

thick is deposited at the membrane center.

The vibration of the film can change the electric field of the 3D-cavity and further modify the cavity frequency. However, the dispersive coupling strength is only on an order of millihertz (mHz). To improve the electromechanical coupling, an H-shaped antenna is deposited on a high-resistance silicon substrate. The Al-film thickness is 120 nm. The antenna chip can trap a cavity electric field inside its central gap area. The detailed size of the antenna is shown in Fig. S1(e).

The metalized SiN-membrane is then placed over the bottom antenna pads. We found that uneven stress distribution will reduce the mechanical Q and introduce spurious mechanical modes. A series of packaging materials and methods were tested, e.g., using indium, GE varnish, and Stycast. Finally, the epoxy resin pillars are used to glue and define the gaps between the upper SiN and lower antenna chips. Such packing methods hold outstanding performances, such as introducing negligible dissipation for cavity and mechanic modes. Even at millikelvin temperature, the epoxy-based encapsulation can still maintain a narrow gap for the mechanically compliant capacitor and will not dramatically change the stress distribution of the SiN membrane. Fig. S1(f) shows the side-view of the assembled mechanically compliant capacitor. The strongest part of the electric field is further localized inside the mechanical capacitor.

In addition to avoiding stress changes caused by packaging materials, we should also take care of the Coulomb force caused by charge accumulation. For the bottom antenna chips, we use high-resistance silicon as its substrate to match the shrinkage to the SiN chips during the cooling process. Any accumulated charge under the membrane will harass the uniform stress distribution and greatly broaden the mechanical linewidth. Compared to the insulating substrate such as sapphire or quartz, the silicon substrate can efficiently avoid charge accumulation. In addition, the particular area of the silicon wafer, directly under the silicon nitride film, is covered by Al film to further remove the charges.

## II. ELECTROMAGNETIC-FIELD DISTRIBUTIONS INSIDE THE 3D-SUPERCONDUCTING CAVITY

In this section, we will use the finite-element simulations to show how the H-shaped antenna can improve the electromechanical couplings. The internal geometric space of the 3D-cavity can be approximately viewed as a cuboid (40 mm$\times$8 mm$\times$14 mm) without considering the chamfers on the edges.

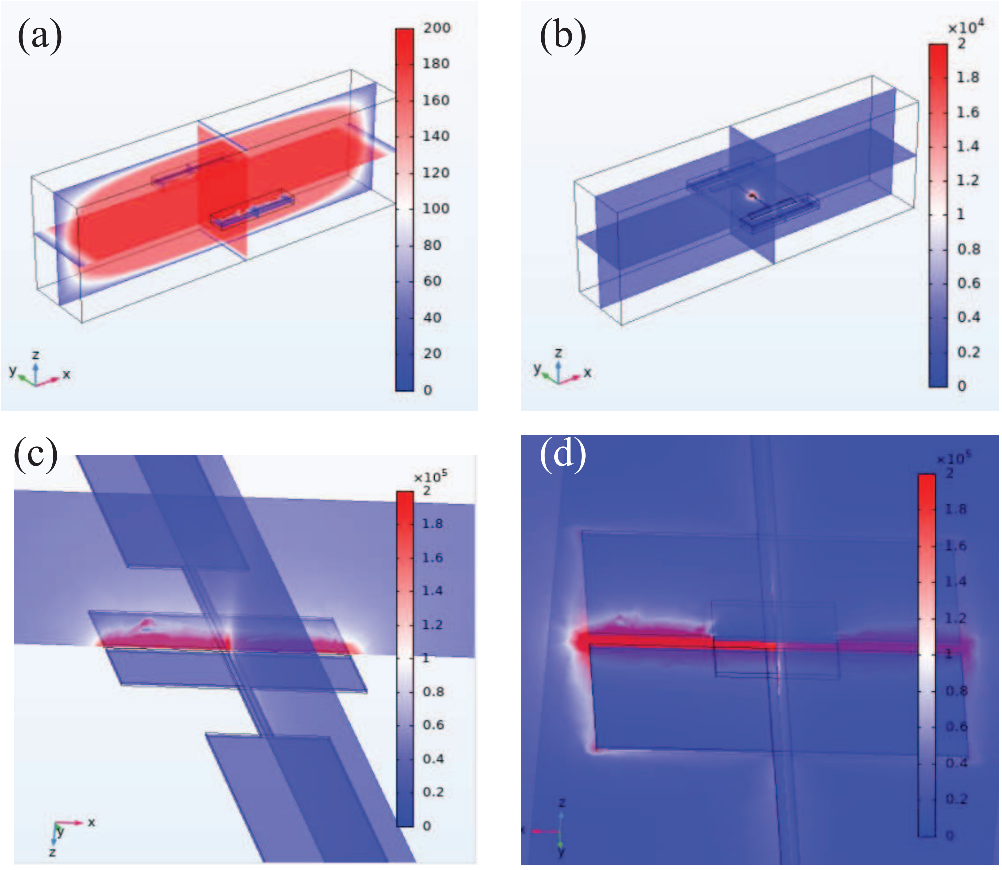


FIG. S2. Electric field distributions are simulated for cases that (a) bare cavity; (b) with bottom antenna. (c) Zoom-in electric field distribution around the antenna gap area and (d) with assembled mechanically compliant capacitor chip.

The cavity electric field distribution for the empty cavity is shown in Fig. S2(a). The electric field is quite uniformly distributed inside the cavity. The maximum electric field with values (200 V/m) locates at the cavity geometric center. The 3D cavity is divided into two symmetrical parts, allowing us to embed the mechanically compliant capacitor chip. When the antenna chip is placed inside the cavity, the electric field is more localized at the cavity center. The maximum value locates at the geometric center of the H-shaped antenna.

The zoom-in electric field distribution is shown in Fig. S2(c). The electric field is enhanced by about three orders of magnitudes compared to the bare cavity case. Fig. S2(d) shows the electric field is further trapped in the gap between the bottom antenna and Al-pad on the SiN membrane. Thus, the single-photon electromechanical coupling can be greatly improved and the coupling strength can arrive at several Hertz level with a technically accessible vacuum gap at one micron.

## III. MEASUREMENT SETUPS

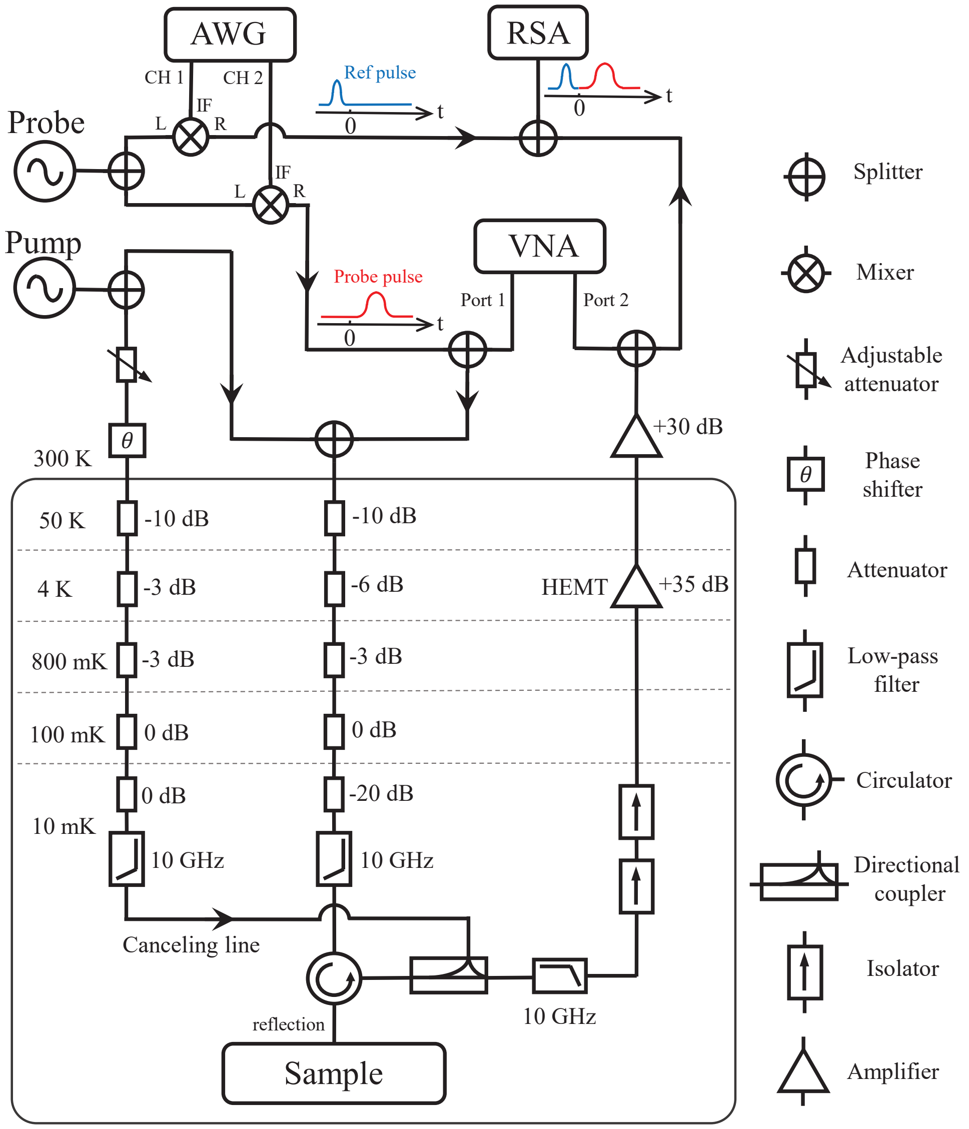


FIG. S3. measurement setups.

The device is mounted on a cold plate at cryogenic temperature around 10 mK in a dilution refrigerator. The Al-block (3D cavity) and Al-films on antenna or SiN chips are superconductors, which supports high-Q microwave cavity resonators. Mechanical linewidth and thermal phonon number can be greatly reduced when device is thermalized to millikelvin (mK) temperature regime. In the dilution refrigerator, three coaxial-cable lines including input, output and

canceling coaxial-cable lines, are used for carrying out the measurements. Through using a circulator, the input and output coaxial-cable lines couple to the same SMA connector of the 3D cavity electromechanical device. A directional coupler is used to combine the canceling line with output line. Thermal noise from the tones at room temperature is suppressed with using attenuators at different temperature stages, and by the attenuation of the coaxial cables. A high electron mobility transistor (HEMT) amplifier is anchored to 4 K, and is isolated from the sample output by two isolators. The pump tone splits into two coherent microwave tones at the room temperature. One is used to pump the cavity-electromechanical device through the input line. The other tone enters the canceling line and meets the reflected pump-tone in the output line. By tuning the amplitude and phase of canceling tone, destructive interference happens and the reflected pump-tone can be effectively canceled to avoid the saturation of the HEMT.

For the measurements of MCPA, a pump tone from a signal generator (Agilent E8257D) and a probe tone from a network analyzer (Agilent N5232A) are combined at room temperature and are transmitted down to the sample. The output signal enters the network analyzer to present the transmission spectrum. It is notable that the mechanical linewidth is quite small, and therefore, for every frequency point of the spectrum, we set the network analyzer at the fixed frequency point more than 100s, to make sure the system into a steady state, then get the system S21 parameter.

To experimentally show the group delay and advance around the $\pi$-phase transition point, a Gaussian-shaped pulse is generated to conduct the time-domain measurement. A continuous-wave pump tone (with frequency $\Omega_c$) is tuned to the fixed red-sideband ($\omega_c - \Omega_c = \omega_m$) and then is sent from a signal generator (Agilent E8257D) to the 3D-cavity. The weak probe field is amplitude-modulated by a Gaussian-shaped envelope generated with an arbitrary waveform generator (Tektronix AWG5014C). We know that the delay is quite sensitive to the frequency of the probe signal, especially around the resonant point. To make the pulse-induced spectral broadening of the probe signal much narrower than mechanical spectrum width, we set the pulse width long enough. For example, at weak pump conditions, we set the Gaussian pulse width to be 2000s long. The emission of this pulse triggers the acquisition of the transmitted probe field via an electronic spectrum analyzer (Tektronix RSA5126B) in zero-span mode. The actual delay of the output pulse is extracted by comparing the center-time difference between the pulse output with and without a pump tone.

## IV. SIMULATION OF THE $\pi$-PHASE TRANSITION

Under red-detuned sideband pump with a frequency close to the lower motional sideband, $\Omega_p = \omega_c - \omega_m$, the optomechanical interaction Hamiltonian can be linearized and becomes beam-splitter like, i.e., $H_{\text{int}}/\hbar = G(a^\dagger b + b^\dagger a)$. In a frame rotating with $\omega_c$, the system total Hamiltonian is given as

$$H/\hbar = \Delta\left(a^\dagger a + b^\dagger b\right) + G\left(a^\dagger b + b^\dagger a\right) + i\sqrt{\eta\kappa}(\varepsilon a^\dagger - \varepsilon^* a). \tag{S1}$$

Taking dissipations into account, the Langevin equation are given as

$$\dot{a} = -\left(i\Delta + \kappa/2\right)a - iGb + \sqrt{\eta\kappa}\varepsilon, \tag{S2}$$

$$\dot{b} = -\left(i\Delta + \gamma_m\right)b - iGa. \tag{S3}$$

Using input-output theory, yields the following expression for the probe field transmission:

$$t = 1 - \frac{\eta\kappa\left(i\Delta + \gamma_m/2\right)}{\left(i\Delta + \gamma_m/2\right)\left(i\Delta + \kappa/2\right) + G^2}. \tag{S4}$$

The amplitude and phase responses are then respectively given as $T = |t|^2$, and $\varphi = \arg(t)$. We now derive the conditions for obtaining the MCPA. The transmission coefficient at zero detuning arrives

$$t_z = t_{\Delta=0} = \frac{G^2 - (\eta - 1/2)\kappa\gamma_m/2}{\kappa\gamma_m/4 + G^2}. \tag{S5}$$

The amplitude at zero detuning is given as

$$T_z = |t_z|^2 = \left|\frac{G^2 - (\eta - 1/2)\kappa\gamma_m/2}{\kappa\gamma_m/4 + G^2}\right|^2. \tag{S6}$$

When all the incident light are absorbed at the cavity resonance, the transmission amplitude at zero detuning is equal to zero, i.e., $T_z = 0$. We then obtain the critical coupling strength $G_{\text{cr}}$ (corresponding $G_c$ in the main text) for the MCPA, i.e.,

$$G_{\text{cr}}^2 = \left(\eta - 1/2\right)\kappa\gamma_m/2. \tag{S7}$$

The optomechanical coupling strengths have been assumed to be real number. Thus, over-coupled external coupling strength (i.e., $\eta$ >1/2) is required in Eq. (S7). Recalling Eq. (S5), it is notable that the imaginary part of $t$ at the zero detuning always equals zero, and the transmission coefficient is real number. Then the phase at the zero detuning is given as

$$\varphi_z = \varphi_{\Delta=0} = \arg(0) = [0, \pi]. \tag{S8}$$

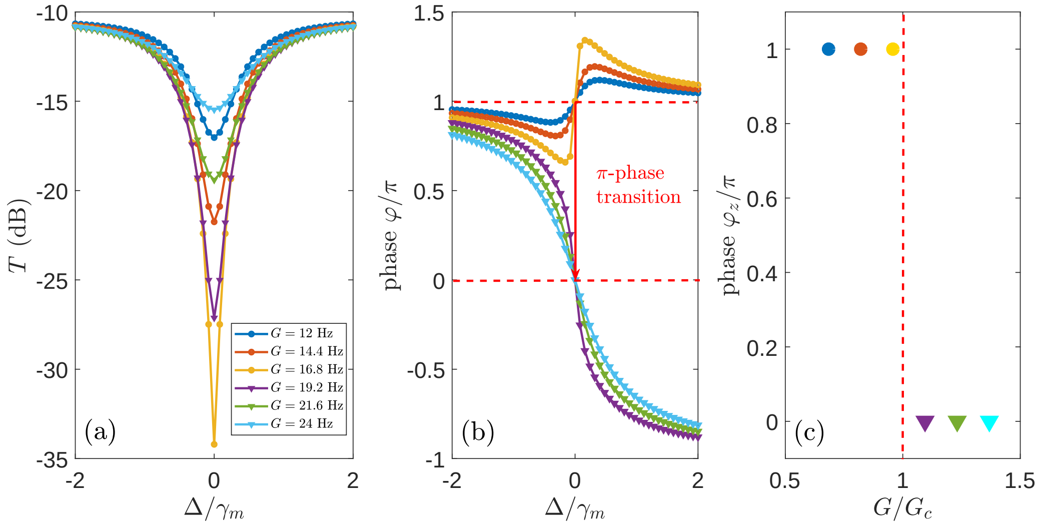


FIG. S4. Red-detuned sideband pump. The amplitude ($T$) and phase response ($\varphi$) with over-coupled external coupling $\eta = 0.651$. (a) Amplitude $T$ and (b) phase $\varphi$ are plotted as functions of detuning $\Delta$. The phase values at zero-detuning ($\varphi_z$) versus coupling strengths are plotted and shown in (c). Coupling strengths $G/2\pi = (12, 14.4, 16.8, 19.2, 21.6, 24)$ Hz are used for calculations. When couplings are smaller (larger) than critical coupling, i.e., $G < G_{cr}$ ($G > G_{cr}$), $T, \varphi$ and $\varphi_z$ curves are marked by filled circles (triangles). At the critical coupling, the phase occurs an abrupt transition from $\pi$ to zero. Other parameters used for the calculation are listed in Table II.

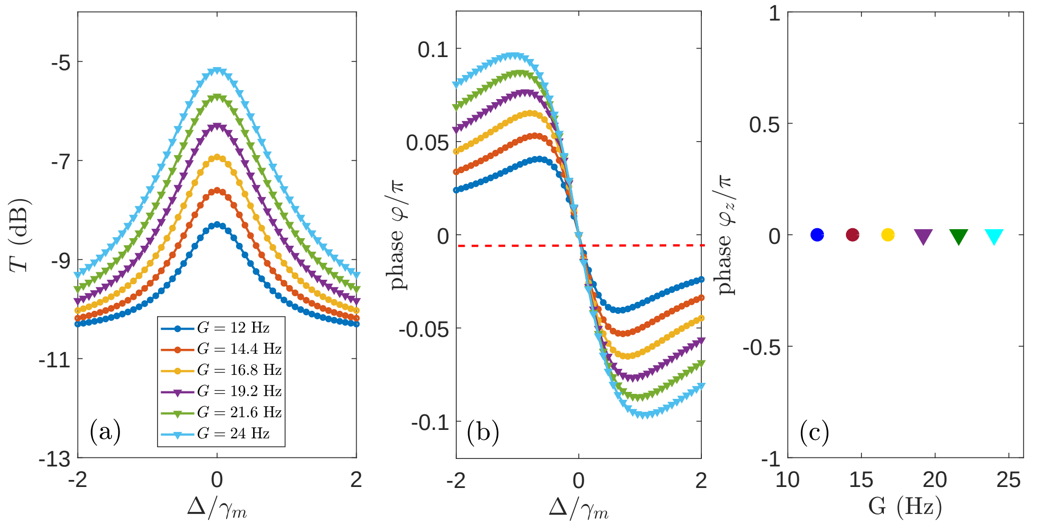


FIG. S5. Red-detuned sideband pump. The amplitude ($T$) and phase response ($\varphi$) with under-coupled external coupling $\eta = 0.451$. Other parameters of this figure are the same as those in Fig. S4.

The above solution indicates that the output laser have two possible phases for any optomechanical coupling strength. To make sure which phase it is for a given $G$, the real part of transmission coefficient $t$ should also be taken into consideration. The phase at zero detuning is given as below:

(i) when $G < |G_{\rm cr}|$, $\varphi_z = \arctan[0/(-|t_z|)] = \arctan\left[\sin(\varphi_z)/\cos(\varphi_z)\right] = \pi$;

(ii) when $G > |G_{\rm cr}|$, $\varphi_z = \arctan\left[0/|t_z|\right] = \arctan\left[\sin(\varphi_z)/\cos(\varphi_z)\right] = 0$.

It is remarkable that when $G = |G_{\rm c}|$, an abrupt transition and a $\pi$-phase shift is observed at such critical coupling strength, at which the MCPA and anti-lasing happens.

To clearly see such transition, $T$, $\varphi$ and $\varphi_z$ are plotted for different coupling strengths and shown in Fig. S4. As shown in Fig. S4(a), absorptions dips are observed for all used coupling strengths. Fig. S4(b) shows the phase evolutions versus detuning $\Delta$ for different coupling strengths. As coupling strength, $G$ passes across $G_{cr}$, the phase response undergoes an abrupt transition with a constant $\pi$-phase shift. Coupling values both above and below $G_{cr}/2\pi = 17.53$ Hz, yield a phase of $\pi$ as the detuning becomes large. As shown in Fig. S4(c), $\varphi_z$ transits from $\pi$ to zero at $G_{cr}$.

With under-coupled cavity (i.e., $\eta$ <1/2), the transmission coefficient at zero-detuning is

$$t_z^w = \frac{G^2 + (1/2 - \eta)\kappa\gamma_m/2}{\kappa\gamma_m/4 + G^2}. \tag{S9}$$

Equation (S9) indicates that $t_z^w$ is always a positive real number for arbitrary positive and real coupling strength $G$. Moreover, the transmission coefficient for the cavity without optomechanical coupling is $t_z^b = (1 - 2\eta)$. The difference between $t_z^w$ and $t_z^b$ is given as

$$R = t_z^w - t_z^b = \frac{8\eta G^2}{4G^2 + \kappa\gamma_m}. \tag{S10}$$

Here, $R$ is always a positive number and monotonically increases with respect to $G$. So, only peaks appear at the cavity resonance and the peak height keeps on raising with increasing the coupling strength $G$ until it arrives unit. As a result, the mechanically induced absorption (or coherent perfect absorption) can not be observed when the external coupling is under-coupled (i.e., $\eta < 1/2$).

When the cavity is under-coupled (e.g., $\eta = 0.451$ in Fig. S5), the amplitude and phase response versus probe detuning $\Delta$ are show in Fig. S5(a) and (b), respectively. With increasing optomechanical coupling $G$, only transparency windows (indicating a transparency) are observed. The phase responses present similar line curves. The phases at cavity resonance, as shown in Fig. S5(c), are always zero. The phase-slope around zero-detuning does not show an abrupt reversal. These behaviors are totally different to those presented in Fig. S4 under an over-coupled external coupling ($\eta = 0.651$).

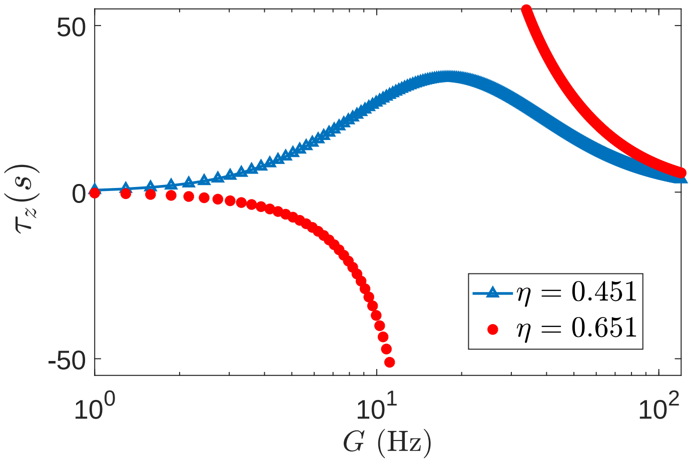


FIG. S6. Red-detuned sideband pump. Group delay at zero-detuning is plotted as a function of coupling strength $G$. Blue-triangle: with a under-coupled external coupling, e.g., $\eta = 0.451$; Red-dots: with an over-coupled external coupling, e.g., $\eta = 0.651$.

At coupling values above and below $G_{cr}$ (corresponding to $G_c$ in the main text), the phase approaches $\pi$ as the detuning becomes large. This only happens if the cavity itself is over-coupled. Whereas, if the external coupling is under-coupled, the phase response for any coupling strength $G$ becomes zero as the detuning becomes large. For a red-detuned pump driving, the cavity will resonantly enhance the anti-stokes scattered sideband photons. Switching from under- to over-coupled external coupling can introduce an entire phase shift of $\pi$ for the anti-stokes photons. As a result, the interference between pump and probe photons changes from destructive interference (corresponding to the observations of OMIT) to constructive interference (corresponding to the observation of OMIA) with beam-splitter like interaction Hamiltonian $H_{\text{int}}/\hbar = G(a^\dagger b + b^\dagger a)$.

The group-delay is closely related to the phase-slope and is given by

$$\tau = \frac{d\varphi}{d\Omega_p} = -\frac{d\varphi}{d\Delta}. \tag{S11}$$

Figure S6 shows the calculated group delay at zero-detuning with under- and over-coupled cavity, respectively. With under-coupling, the group delay is always a positive number (corresponding to slow-light) and shows a maximum value at particular optomechanical coupling. The particular coupling strength to get such maximum group-delay has been in detail discussed in Refs. [2, 3].

However, with over-coupling, e.g., $\eta = 0.651$, the group delay present an infinite discontinuity

and an abrupt transition from group advance to delay occurs at the critical coupling point. The group delay is greatly enhanced and a switchable fast and slow light become possible. Around the singularity, group delay diverges, instead of the normally observed maximum value in group delay in case of under-coupling.

The above discussion is based on a red-detuned sideband pump scheme. We now discuss the probe transmissions under a blue-detuned sideband pump. When driving the cavity at its upper motional sideband, i.e., $\Omega_p = \omega_c + \omega_m$, the interaction Hamiltonian can be written as $H_{\text{int}}/\hbar = G(a^\dagger b^\dagger + ba)$. In a frame rotating with $\omega_c$, the system Hamiltonian is given as

$$H/\hbar = \Delta\left(a^\dagger a + b^\dagger b\right) + G\left(a^\dagger b^\dagger + ba\right) + i\sqrt{\eta\kappa}(\varepsilon a^\dagger - \varepsilon^* a). \tag{S12}$$

Taking dissipations into account, the Langevin equations now become

$$\dot{a} = -\left(i\Delta + \kappa/2\right)a - iGb^\dagger + \sqrt{\eta\kappa}\varepsilon, \tag{S13}$$

$$\dot{b} = -\left(i\Delta + \gamma_m\right)b - iGa^\dagger. \tag{S14}$$

Using input-output theory, we obtain the following expression for the probe field transmission:

$$t = 1 - \frac{\eta\kappa\left(-i\Delta + \gamma_m/2\right)}{\left(-i\Delta + \gamma_m/2\right)\left(i\Delta + \kappa/2\right) - G^2}. \tag{S15}$$

The transmission coefficient at zero detuning is

$$t_z = t_{\Delta=0} = \frac{G^2 - (1/2 - \eta)\kappa\gamma_m/2}{G^2 - \kappa\gamma_m/4}. \tag{S16}$$

The amplitude at zero detuning is given as

$$T_z = |t_z|^2 = \left|\frac{G^2 - (1/2 - \eta)\kappa\gamma_m/2}{G^2 - \kappa\gamma_m/4}\right|^2. \tag{S17}$$

When all the incident light is absorbed at the cavity resonance, the transmission amplitude at zero detuning is equal to zero, i.e., $T_z = 0$. We then obtain the critical coupling strength $G_{\text{cb}}$ for the MCPA, i.e.,

$$G_{\text{cb}}^2 = \left(1/2 - \eta\right)\kappa\gamma_m/2. \tag{S18}$$

Opposite to Eq.(S7), under-coupled cavity (i.e., $\eta$ <1/2) is required for Eq. (S18) to be solvable. The transmission spectrum can now be changed from absorption to amplification by tuning the pump power [4]. We now discuss the accompanying phase responses when CPA occurs at a critical coupling $G_{cb}$. The probe transmission is given in Equation. (S16). At the zero detuning,

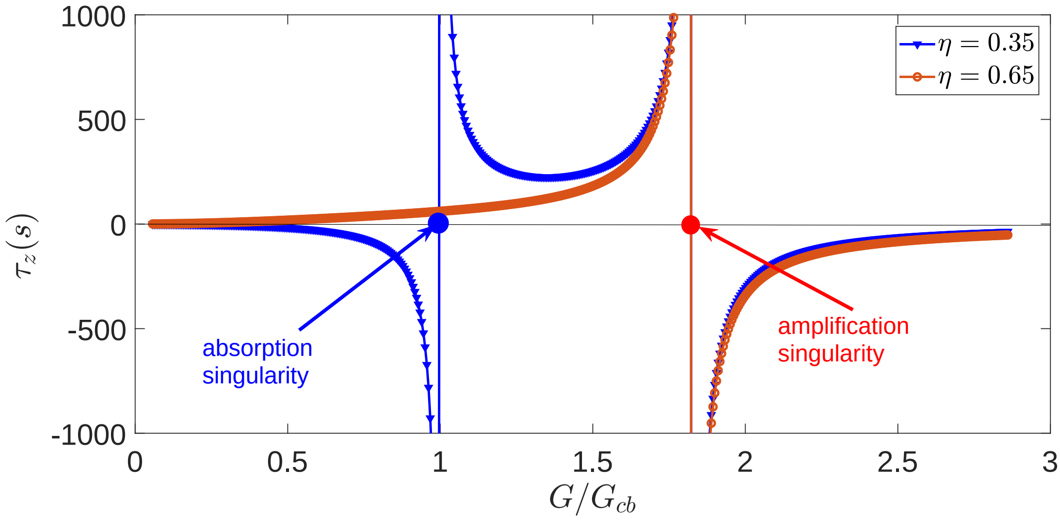


FIG. S7. Blue-detuned sideband pump. Group delay at zero-detuning is plotted as a function of coupling strength $G$. Blue-triangle: with a under-coupled external coupling, e.g., $\eta = 0.35$; Red-dots: with an over-coupled external coupling, e.g., $\eta = 0.65$.

TABLE I. Interference type and phases trends

| | under-coupled ($\eta < 1/2$) | over-coupled ($\eta > 1/2$) |
|---|---|---|
| blue-detuned pump | constructive interference (OMIA)<br>phase tends to zero | destructive interference (OMIT)<br>phase tends to $\pi$ |
| red-detuned pump | destructive interference (OMIT)<br>phase tends to zero | constructive interference (OMIA)<br>phase tends to $\pi$ |

the imaginary part of $t$ always equals zero, and the transmission coefficient is real number. Then the phase at the zero detuning is given as

$$\varphi_z = \varphi_{\Delta=0} = \arg(0) = [0, \pi]. \quad \text{(S19)}$$

The above solution indicates that the output laser has two possible phases for any optomechanical coupling strength. To make sure which phase it is for a given $G$, the real part of transmission coefficient $t$ should also be taken into consideration. The phase at zero detuning is determined as follows:

(i) when $G < |G_{\mathrm{cb}}|$, $\varphi_z = \arctan[0/|t_z|] = \arctan[\sin(\varphi_z) / \cos(\varphi_z)] = 0$;

(ii) when $G > |G_{\mathrm{cb}}|$, $\varphi_z = \arctan[0/-|t_z|] = \arctan[\sin(\varphi_z) / \cos(\varphi_z)] = \pi$.

It is remarkable that when $G = |G_{\mathrm{cb}}|$, an abrupt transition and a $\pi$-phase shift is observed at such

critical coupling strength. The $\pi$-phase transition now is jumped from zero to $\pi$, whereas, for red-detuned sideband pump, phase transits from $\pi$ to zero, as the probe field detuning is increased.

The $\pi$-phase transition under the blue-detuned sideband is also mediated by the MCPA. In addition to the above-discussed zeros of $t_z$, the transmission rate given in Eq. (S16) also indicates poles with large amplification. The probe photon number approaches infinite when coupling strength arrives at $G_l = \sqrt{\kappa\gamma_m/4}$. It is worth noting that $\pi$-phase transition also occurs when $G$ is increased across $G_l$, and the phase is transited from $\pi$ to zero. Actually, the phase at zero-detuning can be obtained as below:

(i) when $G_{cb} < G < G_l$ $|G_1|$, $\varphi_z = \arctan[0/(-|t_z|)] = \arctan\left[\sin\left(\varphi_z\right)/\cos\left(\varphi_z\right)\right] = \pi$;

(ii) when $G > |G_1|$, $\varphi_z = \arctan\left[0/\left|t_z\right|\right] = \arctan\left[\sin\left(\varphi_z\right)/\cos\left(\varphi_z\right)\right] = 0$.

The group delay at zero-detuning is plotted as a function of $G$ and shown in Fig. S7. When the external coupling is under-coupled, MCPA mediates a group delay singularity and fast light can be switched to slow light when $G$ crossing $G_{cb}$. Further increasing $G$, another group delay singularity accompanied by probe amplification in its amplitude is observed. Slow light could be switched to fast light when $G$ is over $G_l$. So, when coupling strength arrives at $G_l$, the amplification singularity will also introduce the $\pi$-phase transition in its phase response and further flip the phase slope at cavity resonance. A group delay approaching infinite and an abrupt transition between fast-slow light is observed. Compared to the singularity mediated by CPA (called absorption singularity), the singularity at $G_l$ is with amplification (called amplification singularity). Thus, the amplification singularity would allow us to realize a large group delay without additional absorption.

Table I summarizes the interference type under different external coupling and driving schemes. Around the cavity resonance, the phase tends to be zero, or $\pi$ is also clarified. In conclusion, one can switch between constructive and destructive interference by changing the driving between blue-detuned and red-detuned pumps or modifying the external coupling condition.

## V. DEVICE PARAMETERS AND THE OPTOMECHANICAL COUPLING STRENGTH

The amplitude and phase responses are shown in Fig. S4(a) and (b), respectively. Fitted using $T = |t|^2$, and $\varphi = \arg(t)$, the system parameters and optomechanical coupling strength $G$ are given in Table. II. The mechanical frequency and linewidth are further measured through the power spectral density of the thermal mechanical motion. The membrane mechanical resonator frequency is $\omega_m/2\pi$=755.54 kHz with linewidth $\gamma_m/2\pi = 9.7$ mHz, corresponding $Q_m = 7.78 \times 10^7$.

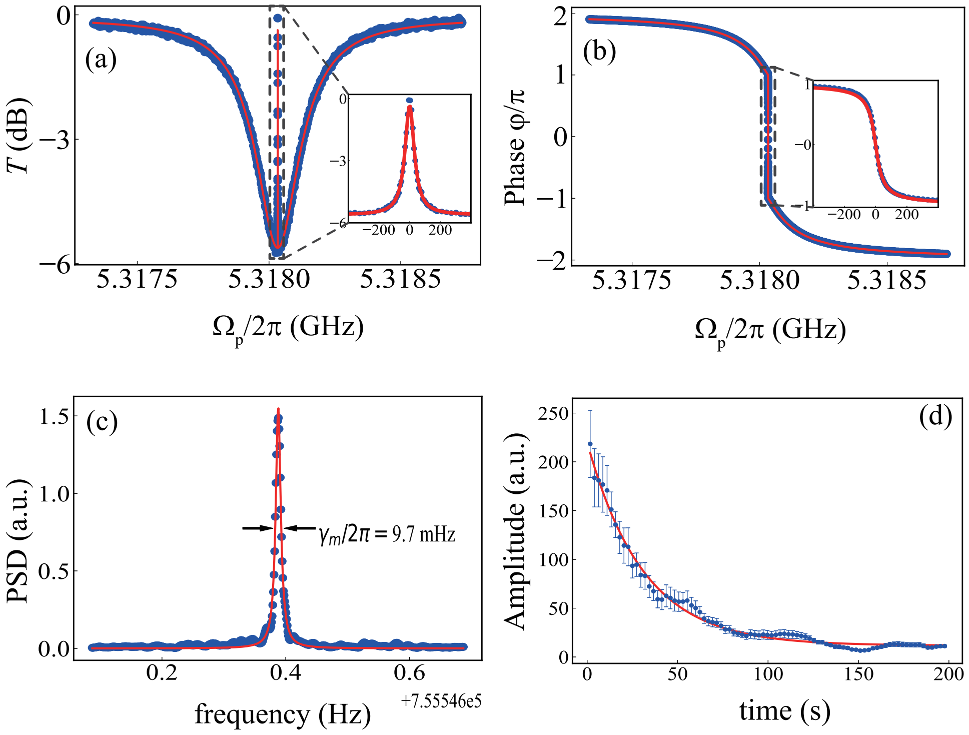


FIG. S8. Amplitude (a) and phase (b) responses of the OMIT. The mechanical power density spectrum (c) and (d) ringdown measurement. Blue: data; Red; fit.

TABLE II. calibrated system parameters

| $\kappa/2\pi$ | $\eta$ | $G/2\pi$ | $\gamma_m/2\pi$ |
|---|---|---|---|
| 420 kHz | 0.651 | 176.8 Hz | 9.7 mHz |

## VI. GROUP DELAY MEASUREMENTS BY THE VNA

The group delay extracted by measuring Gaussian-shaped pulse propagating has been shown in Fig. 5 in the main text. As the examples, the group delay under three typical coupling strengths, e.g., $G = 11.87$ Hz (on the left of $G_c$), $G = 23.93$ Hz (on the right of $G_c$), and $G = 155.1$ Hz (in the transparency regime), are obtained by the pulsed measurements. Meanwhile, the group delay could also be measured by using a continuous probe-tone generated by the VNA. The corresponding group delay is shown in Fig. S9. The obtained group delay measured by the VNA agrees well with the pulsed measurements shown in Fig. 5 in the main text.

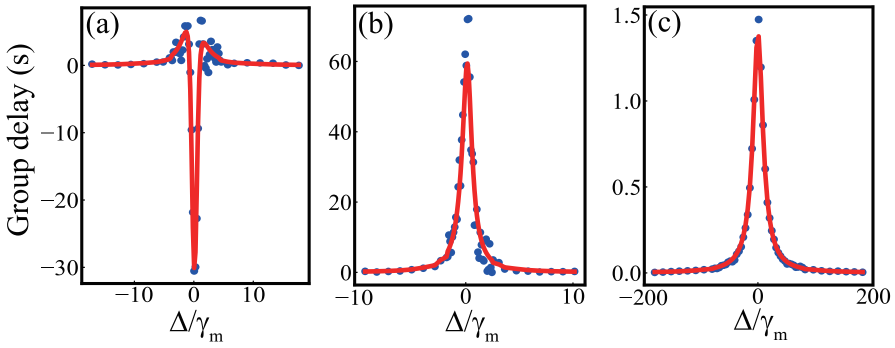


FIG. S9. Group delay measured by using a continuous probe-tone generated and analysed by the VNA. The coupling strength are $G/2\pi = 11.87$ Hz for (a), $G/2\pi = 23.93$ Hz for (b), and $G/2\pi = 155.1$ Hz for (c), respectively. Blue: data; Red; fit.

* mika.sillanpaa@aalto.fi

† litf@tsinghua.edu.cn

[1] A. Noguchi, R. Yamazaki, M. Ataka, H. Fujita, Y. Tabuchi, T. Ishikawa, K. Usami, and Y. Nakamura, Ground state cooling of a quantum electromechanical system with a silicon nitride membrane in a 3D loop-gap cavity, New Journal of Physics **18**, 103036 (2016).

[2] A. H. Safavi-Naeini, T. P. Alegre, J. Chan, M. Eichenfield, M. Winger, Q. Lin, J. T. Hill, D. E. Chang, and O. Painter, Electromagnetically induced transparency and slow light with optomechanics, Nature **472**, 69 (2011).

[3] X. Zhou, F. Hocke, A. Schliesser, A. Marx, H. Huebl, R. Gross, and T. J. Kippenberg, Slowing, advancing and switching of microwave signals using circuit nanoelectromechanics, Nature Physics **9**, 179 (2013).

[4] F. Hocke, X. Zhou, A. Schliesser, T. J. Kippenberg, H. Huebl, and R. Gross, Electromechanically induced absorption in a circuit nano-electromechanical system, New Journal of Physics **14**, 123037 (2012).
